# Supplementary material for: Modified Gravity and Regular Black Hole Models
Source: arXiv:2511.12902 source file (2025-11-17)
Supplement: Supplementary file 4 [file AppendixD.tex]

\chapter{Higher Dimensional pencil-like sources and their ultrarelativistic limit}
\label{app:Higher-Dim}

\section{Stationary Electromagnetic Field of Extended Objects}\label{sec1.2}

Since Maxwell’s equations are linear, the electromagnetic field of extended charged and/or magnetized objects can be obtained by superposing the solutions derived for corresponding point-like sources. That is, the fields can be expressed as integrals involving the Green function multiplied by the current distributions that appear on the right-hand side of Maxwell’s equations. In many cases, when the current distributions possess sufficient symmetry, these integrals can be computed explicitly (see, e.g., \cite{Jackson}). In this appendix, we present the field expressions for two special configurations that will be important for our later discussion of ultrarelativistic objects. Specifically, we consider electrically charged and magnetized pencil-like configurations, both of which are assumed to have vanishingly small transverse dimensions.

We analyze these objects from the perspective of two reference frames: the rest frame, where the object is stationary, and a frame in which the object moves with constant velocity. To distinguish them, we denote the rest frame by $\bar{S}$ and the moving frame by $S$. Accordingly, all quantities in the rest frame will carry a bar, while those in the moving frame will not. 

Let $\bar{L}$ be the length of the pencil as measured in the rest frame. We choose coordinates $\bar{X}^{\mu}$ in $\bar{S}$ such that one spatial axis aligns with the pencil’s longitudinal direction, denoted by $\bar{\xi}$. The coordinates orthogonal to this axis are labeled $\vec{x}_{\perp}$, so that
\begin{align}
\bar{X}^{\mu} = (\bar{t}, \bar{\xi}, \vec{x}_{\perp})\, .
\end{align}
We place the origin of the coordinate system such that the pencil’s endpoints lie at $\bar{\xi} = \pm \bar{L}/2$. In subsequent sections, we will perform a boost in the $\bar{\xi}$-direction.

We consider two types of pencils: one that is uniformly electrically charged with total charge $\bar{q}$, and another that is uniformly magnetized with total magnetic moment $\bar{m}$. We refer to these configurations as the $q$-pencil and $m$-pencil, respectively.

\subsection{Field of a q-pencil in Its Rest Frame}

We begin with the $q$-pencil, assuming a uniform charge density along its length. If $\bar{q}$ is the total charge and $\bar{L}$ the pencil’s length, then the charge density is given by:
\begin{align}
\bar{\lambda} = \frac{\bar{q}}{\bar{L}} \delta^{(2)}(\vec{x}_{\perp}) \, \Theta(\bar{\xi} | -\bar{L}/2, \bar{L}/2)\, ,
\end{align}
and the associated 4-current $\bar{j}^{\mu}$ is:
\begin{align}
\bar{j}^{\mu} = \delta^{\mu}_{\bar{t}} \bar{\lambda}\, .
\end{align}
Here, $\Theta(x | x_-, x_+)=\theta(x - x_-) \theta(x_+ - x)$ is a step function that equals 1 in the interval $(x_-, x_+)$ and vanishes elsewhere.

In the Coulomb gauge $\partial_j A^j = 0$, we may choose the vector potential in the form:\footnote{$\mathbf{A}$, as a differential form, is Lorentz-invariant. For this reason, we omit the bar notation on bold-faced symbols here and in what follows.}
\begin{align}\label{POT_T}
\mathbf{A} \equiv \bar{A}_{\mu} d\bar{X}^{\mu} = \bar{\phi} \, d\bar{t}\, .
\end{align}
Solving the field equation for the potential $\bar{\phi}$,
\begin{align}
\Delta \bar{\phi} = -\bar{\lambda}\, ,
\end{align}
one obtains:
\begin{align}\label{PP}
\bar{\phi}(\bar{\xi}, \rho) = \frac{\bar{q}}{4\pi \bar{L}} \int_{-\bar{L}/2}^{\bar{L}/2} \frac{d\bar{\xi}'}{\sqrt{(\bar{\xi} - \bar{\xi}')^2 + \rho^2}}\, ,
\end{align}
where $\rho = |\vec{x}_{\perp}|$. Evaluating the integral yields:
\begin{align}
\bar{\phi}(\bar{\xi}, \rho) = \frac{\bar{q}}{4\pi \bar{L}} \ln \left( \frac{ \bar{\xi}_+ + \sqrt{\bar{\xi}_+^2 + \rho^2} }{ \bar{\xi}_- + \sqrt{\bar{\xi}_-^2 + \rho^2} } \right)\, ,
\end{align}
where we have defined $\bar{\xi}_{\pm} = \bar{\xi} \pm \bar{L}/2$ for convenience.

\subsection{Field of an m-pencil in Its Rest Frame}

Let us now introduce polar coordinates $\{\rho, \varphi\}$ in the plane orthogonal to the pencil. In these coordinates, the Minkowski metric becomes:\footnote{Note that the angular component $\partial_\varphi$ does not represent a unit basis vector, but rather has norm $\rho$. Care is required when comparing our results to those in the literature, which sometimes use orthonormal frames with the unit vector $\hat{\varphi} = \partial_\varphi/\rho$.}
\begin{align}
ds^2 = -d\bar{t}^2 + d\bar{\xi}^2 + d\rho^2 + \rho^2 d\varphi^2\, .
\end{align}
To determine the field of the $m$-pencil, we begin with a finite-radius solenoid of current density:
\begin{align}
\begin{split}
\mathbf{J} &= \bar{J}_{\varphi} d\varphi\, , \\
\bar{J}_{\varphi} &= \frac{\bar{m}}{\pi \bar{L} R} \delta(\rho - R) \, \Theta(\bar{\xi} | -\bar{L}/2, \bar{L}/2)\, .
\end{split}
\end{align}
Here, $R$ is the solenoid’s radius, $\bar{L}$ its length in the rest frame $\bar{S}$, and $\bar{m}$ its total magnetic moment, which is proportional to the enclosed magnetic flux.

Since the magnetic field is static and axially symmetric, we can write the vector potential as $\bar{\mathbf{A}} \equiv \bar{A}_{\mu} d\bar{X}^{\mu} = \bar{A}_{\varphi} d\varphi$. In the limit $R \to 0$, the potential $\bar{A}_{\varphi}$ becomes \cite{Boos_2021}:
\begin{equation}\label{AF}
\bar{A}_{\varphi} = \frac{\bar{m}}{4\pi \bar{L}} \left( \frac{\bar{\xi}_+}{\sqrt{\bar{\xi}_+^2 + \rho^2}} - \frac{\bar{\xi}_-}{\sqrt{\bar{\xi}_-^2 + \rho^2}} \right)\, .
\end{equation}
As before, we define $\bar{\xi}_{\pm} = \bar{\xi} \pm \bar{L}/2$. It can also be shown that expression \eqref{AF} matches the field generated by a monopole--anti-monopole pair located along the $\bar{\xi}$-axis and separated by a distance $\bar{L}$.

\section{On the source of static magnetized sources in an arbitrary number of dimensions}

In order to obtain the solutions for equations \eqref{field-eq-highdimg-maxwell}, one may consider the following external current:
\begin{align}\label{appCUR}
j{}^\mu = \delta{}^\mu_t \, q \, \delta{}^{(d)}(\mathbf{x}) + \delta{}^\mu_i \, M{}^{ik} \, \partial_k \delta{}^{(d)}(\mathbf{x}) \, ,
\end{align}
where \( q \) denotes the electric charge of a point particle, and \( M_{ik} = -M_{ki} \) is a constant antisymmetric matrix characterizing the particle’s intrinsic magnetic moment.

Let us write \( d = 2k + \sigma \), where \( \sigma = 0 \) for even \( d \), and \( \sigma = 1 \) for odd \( d \). Any antisymmetric \( d \times d \) matrix can be brought to a block-diagonal form through an orthogonal transformation in \( d \)-dimensional space~\cite{Gantmacher:1959:TMa,Gantmacher:1959:TMb,prasolov1996}. In the corresponding Darboux coordinate system, the matrix \( \mathbf{M} \) takes the canonical form (see~\cite{pinedo2022gravitational}):
\begin{equation}\label{MMMM}
\mathbf{M} = \begin{bmatrix}
    \mathbf{m}_1 & 0 & \dots  & 0 & 0 \\
    0 & \mathbf{m}_2 & \dots  & 0 & 0 \\
    \vdots  & \vdots  & \ddots  & \vdots  & \vdots \\
    0 & \dots  & \dots & \mathbf{m}_k & 0 \\
    0 & 0 & \dots  & 0 & 0 \\
\end{bmatrix} \, ,
\end{equation}
where each \( \mathbf{m}_a \) is a \( 2 \times 2 \) block of the form
\begin{equation}
\mathbf{m}_a = \begin{bmatrix}
    0 & m_a \\
   -m_a & 0 \\
\end{bmatrix} \, .
\end{equation}
The final row and column of zeros appear only in the case \( \sigma = 1 \) and are absent when \( \sigma = 0 \). The parameters \( m_a \) represent the independent components of the magnetic moment. In four spacetime dimensions (\( d = 3 \)), only one such block appears, corresponding to a single magnetic moment component.

\section{Charged and magnetized pencil-like sources in the infinite derivative Maxwell model}

In this section, we will repeat the same steps from the previous sections, but we will now apply the infinite derivative version of the Maxwell equations.

\subsection{Pencil-like Sources}\label{sect2.6}

Now we turn to four-dimensional pencil-type configurations. To describe such objects, we designate one spatial coordinate, denoted by $ \bar{\xi} $, as the direction along the pencil. We organize the spacetime coordinates as $ \bar{X}^\mu = (\bar{t}, \bar{\xi}, \mathbf{x}_\perp) $, and write the flat metric as
\begin{align}
d s^2 = -d\bar{t}^2 + d\bar{\xi}^2 + d\mathbf{x}_\perp^2 \, .
\end{align}
As before, quantities evaluated in the rest frame of the source $ \bar{S} $ are indicated with bars. Since the transverse space orthogonal to the pencil direction $ \bar{\xi} $ has dimension $ d-1 = 2$, then the transverse metric is
\begin{equation}
d\mathbf{x}_\perp^2 = dx^2 +  dy^2\, .
\end{equation}

We can therefore introduce polar coordinates $ \{ \rho, \varphi \} $ in the plane spanned by these coordinates, related to the Cartesian coordinates by
\begin{equation}
x = \rho \cos \varphi, \quad y = \rho \sin \varphi \, .
\end{equation}
Assuming that the pencil lies in the $\bar{\xi} = z$ direction. In these coordinates, the metric becomes
\begin{align}
d s^2 = -d\bar{t}^2 + d\bar{\xi}^2 + d\rho^2 + \rho^2d\varphi^2 ,
\end{align}
and the field of a point-like source, equation~\eqref{APOT2}, takes the form
\begin{align}
\label{eq:a:pre-boost}
\bar{A}_\mu d\bar{X}^\mu = \bar{q} \, \mathcal{G}_3(\bar{r}) \, d\bar{t} - 2\pi \, \mathcal{G}_{5}(\bar{r}) \bar{m} \rho^2 \, d\varphi \, , \nonumber \\
\bar{r}^2 = \bar{\xi}^2 + \mathbf{x}_\perp^2 = \bar{\xi}^2 + \rho^2 \, .
\end{align}

We now construct a solution for an extended, stationary source distributed along the $ \bar{\xi} $-direction. For simplicity, we consider charged and/or magnetized pencils with delta-function profiles in the transverse directions, while allowing arbitrary profiles along $ \bar{\xi} $. Let $ \bar{\lambda}(\bar{\xi}) $ and $ \bar{\mu}(\bar{\xi}) $ denote the charge and magnetic moment densities along the pencil, respectively. The associated conserved current is then
\begin{align}
j^\mu = \delta^\mu_{\bar{t}} \lambda(\bar{\xi}) \delta^{(2)}(\mathbf{x}_\perp) + \delta^\mu_i \bar{\mu}^{ik}(\bar{\xi}) \, \partial_k \delta^{(2)}(\mathbf{x}_\perp) \, .
\end{align}
Where the magnetic moment density is
\begin{equation}
\bar{\mu}_{ik}(\bar{\xi}) =  \mu(\bar{\xi}) \, \epsilon_{ij} \, .
\end{equation}
And we impose that the matrix $\bar{\mu}^{ik}$ has no components along $\bar{\xi}$. The resulting conserved current takes the form
\begin{equation}\label{currentPencil}
j^\mu = \left[ \delta^\mu_t \lambda(\bar{\xi}) + \mu(\bar{\xi}) \, \epsilon^{\mu j} \, \partial_j \right] \delta^{(2)}(x_\perp) \, .
\end{equation}

The total charge $ \bar{q} $ and magnetic moments $ \bar{m}_a $ are obtained by integrating these densities:
\begin{align}
\bar{q} = \int_{-\infty}^\infty d\bar{\xi} \, \bar{\lambda}(\bar{\xi}) \, , \quad
\bar{m} = \int_{-\infty}^\infty d\bar{\xi} \, \bar{\mu}(\bar{\xi}) \, .
\end{align}
If the pencil has finite length, the integrals are taken over a corresponding finite interval.

Finally, the vector potential $ \mathbf{A} $ generated by the current \eqref{currentPencil} has the components
\begin{align}
A_t &= \int_{-\infty}^\infty d\bar{\xi}' \, \lambda(\bar{\xi}') \, \mathcal{G}_3(r) \, , \\
A_\varphi &= -2\pi \int_{-\infty}^\infty d\bar{\xi}' \, \mathcal{G}_{5}(r) \mu(\bar{\xi}') \rho^2 \, ,
\end{align}
where
\begin{align}
r^2 = (\bar{\xi} - \bar{\xi}')^2 + \rho^2 \, ,
\end{align}
We will revisit this configuration when performing the boost of the pencil.

\subsection{Pencil-like sources in higher dimensions}

We now consider a special class of higher-dimensional extended sources that generalize the four-dimensional pencil-type configurations. The space transverse to the pencil direction $\bar{\xi}$ has dimension $d-1 = 2n + \epsilon$, where $\epsilon = 0$ if $d$ is odd and $\epsilon = 1$ if $d$ is even. The corresponding transverse metric is
\begin{equation}
d\mathbf{x}_\perp^2 = \sum_{j=1}^{d-1} (d x_\perp^j)^2 \, .
\end{equation}

Within this transverse space, we choose $n$ mutually orthogonal two-dimensional planes $\Pi_a$, labeled by $a = 1, \ldots, n$. When $d$ is odd ($\epsilon = 0$), these $n$ planes span the entire transverse space. For even $d$ ($\epsilon = 1$), there is one additional orthogonal direction, denoted by $z$. This decomposition is illustrated in Figure~\eqref{fig:darboux}.

Although the choice of planes $\Pi_a$ is not unique in general, we assume they are aligned with the eigenspaces of a given antisymmetric matrix $\mathbf{M}$. This guarantees that the current in equation~\eqref{appeq:ultrarelativistic-pencil} has support only in directions orthogonal to $\bar{\xi}$. In four spacetime dimensions ($d = 3$, so $n = 1$), this condition implies that the magnetic moment vector is aligned with the pencil axis $\bar{\xi}$—a condition that we naturally generalize to higher dimensions.

We introduce Darboux coordinates adapted to the planes $\Pi_a$, labeling each pair as $(y_a, \hat{y}_a)$, so that the metric becomes
\begin{equation} \label{Pcoor}
ds^2 = -d\bar{t}^2 + d\bar{\xi}^2 + \sum_{a=1}^n (dy_a^2 + d\hat{y}_a^2) + \epsilon \, dz^2 \, .
\end{equation}

\begin{figure}[!hbt]
    \centering
    \vspace{10pt}
    \includegraphics[width=0.7\textwidth]{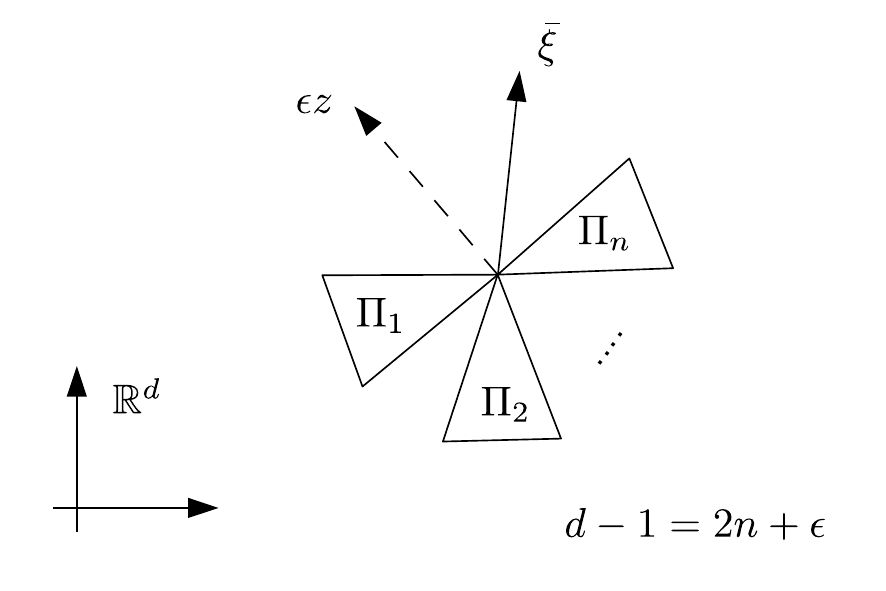}
    \caption{Darboux decomposition of $d$-dimensional space into $n$ mutually orthogonal planes $\Pi_a$ and an additional $z$-direction when $\epsilon = 1$ \cite{Boos_2020}.}
    \label{fig:darboux}
\end{figure}

We further introduce polar coordinates $\{\rho_a, \varphi_a\}$ in each plane $\Pi_a$, related to the Cartesian coordinates by
\begin{equation}
y_a = \rho_a \cos \varphi_a, \quad \hat{y}_a = \rho_a \sin \varphi_a \, .
\end{equation}
In these coordinates, the metric becomes
\begin{align}
ds^2 = -d\bar{t}^2 + d\bar{\xi}^2 + \sum_{a=1}^n (d\rho_a^2 + \rho_a^2 d\varphi_a^2) + \epsilon \, dz^2 \, ,
\end{align}
and the field of a point-like source, equation~\eqref{appAPOT2}, takes the form
\begin{align}
\bar{A}_\mu d\bar{X}^\mu = \bar{q} \, \mathcal{G}_d(\bar{r}) \, d\bar{t} - 2\pi \, \mathcal{G}_{d+2}(\bar{r}) \sum_{a=1}^n \bar{m}_a \rho_a^2 \, d\varphi_a \, , \nonumber \\
\bar{r}^2 = \bar{\xi}^2 + \mathbf{x}_\perp^2 = \bar{\xi}^2 + \sum_{a=1}^n \rho_a^2 + \epsilon z^2 \, .
\end{align}

Next, we construct a solution for an extended, stationary source distributed along the $\bar{\xi}$-direction. For simplicity, we consider charged and/or magnetized pencils with delta-function profiles in the transverse directions, while allowing arbitrary profiles along $\bar{\xi}$. Let $\bar{\lambda}(\bar{\xi})$ and $\bar{\mu}_a(\bar{\xi})$ denote the charge and magnetic moment densities along the pencil, respectively. The associated conserved current is
\begin{align}
j^\mu = \delta^\mu_{\bar{t}} \lambda(\bar{\xi}) \delta^{(d-1)}(\mathbf{x}_\perp) + \delta^\mu_i \bar{\mu}^{ik}(\bar{\xi}) \, \partial_k \delta^{(d-1)}(\mathbf{x}_\perp) \, .
\end{align}

We impose two additional assumptions:
\begin{itemize}
    \item The matrix $\bar{\mu}^{ik}(\bar{\xi})$ has no components along $\bar{\xi}$: $\bar{\mu}^{i\bar{\xi}}(\bar{\xi}) = 0$.
    \item Its eigenspaces—mutually orthogonal two-planes—are parallel transported along the $\bar{\xi}$-direction.
\end{itemize}
These conditions ensure that Darboux coordinates $(y_a, \hat{y}_a)$ can be consistently used across the pencil. In each plane $\Pi_a$, we introduce the orthonormal vectors
\begin{equation}
\mathbf{e}^{(a)} = \partial_{y^a}, \quad \mathbf{e}^{(\hat{a})} = \partial_{\hat{y}^a} \, ,
\end{equation}
with corresponding dual one-forms
\begin{equation}
\boldsymbol{\omega}^{(a)} = dy^a, \quad \boldsymbol{\omega}^{(\hat{a})} = d\hat{y}^a \, .
\end{equation}
The volume element in the $a$-th Darboux plane is then
\begin{equation}
\epsilon^{(a)} = \boldsymbol{\omega}^{(a)} \wedge \boldsymbol{\omega}^{(\hat{a})} \, .
\end{equation}
In this basis, the magnetic moment density takes the form
\begin{equation}
\bar{\mu}_{ik}(\bar{\xi}) = \sum_{a=1}^n \mu_a(\bar{\xi}) \, \epsilon^{(a)}_{ij} \, .
\end{equation}
The resulting conserved current becomes
\begin{equation}\label{currr}
j^\mu = \left[ \delta^\mu_t \lambda(\bar{\xi}) + \sum_{a=1}^n \mu_a(\bar{\xi}) \, \epsilon^{(a)\mu j} \, \partial_j \right] \delta^{(d-1)}(x_\perp) \, .
\end{equation}

Here, $\lambda(\bar{\xi})$ and $\mu_a(\bar{\xi})$ describe the charge and magnetic moment densities along the pencil. The total charge $\bar{q}$ and the magnetic moments $\bar{m}_a$ are given by
\begin{align}
\bar{q} = \int_{-\infty}^\infty d\bar{\xi} \, \bar{\lambda}(\bar{\xi}) \, , \quad
\bar{m}_a = \int_{-\infty}^\infty d\bar{\xi} \, \bar{\mu}_a(\bar{\xi}) \, .
\end{align}

The vector potential $\mathbf{A}$ generated by the current~\eqref{currr} then reads
\begin{align}
A_t &= \int_{-\infty}^\infty d\bar{\xi}' \, \lambda(\bar{\xi}') \, \mathcal{G}_d(r) \, , \\
A_a &= -2\pi \int_{-\infty}^\infty d\bar{\xi}' \, \mathcal{G}_{d+2}(r) \sum_{a=1}^n \mu_a(\bar{\xi}') \rho_a^2 \, ,
\end{align}
with
\begin{align}\label{app-radiusdef}
r^2 = (\bar{\xi} - \bar{\xi}')^2 + \mathbf{x}_\perp^2 \, , \quad
\mathbf{x}_\perp^2 = \sum_{a=1}^n \rho_a^2 + \epsilon z^2 \, .
\end{align}

\section{Boost Transformation and Penrose Limit}

We are now ready to examine the electromagnetic and gravitational fields of ultrarelativistic pencils of finite length. We demonstrate that these fields can be obtained by boosting the previously derived solutions for stationary sources. To this end, we first express the stationary solutions in an inertial frame $S$ moving with velocity $\beta = v/c$ relative to the rest frame $\bar{S}$, and then take the limit $\beta \to 1$. To obtain finite results in this ultrarelativistic limit, the source parameters in the rest frame must be rescaled appropriately. This rescaling depends on the spin of the field and differs between the electromagnetic and gravitational cases. In the gravitational theory, one keeps the total energy in the boosted frame fixed rather than the mass in the rest frame.

Penrose showed that such a limiting process is valid beyond linearized gravity. In his seminal work \cite{Penrose1976}, he described the procedure as follows:
\begin{quote}
We envisage a succession of observers travelling in the spacetime $\mathcal{M}$ whose world lines approach the null geodesic $\gamma$ more and more closely; so we picture these observers as travelling with greater and greater speeds, approaching that of light. As their speeds increase they must correspondingly recalibrate their clocks to run faster and faster (assuming that all spacetime measurements are referred to clock measurements in the standard way), so that in the limit the clocks measure the affine parameter along $\gamma$. (Without clock recalibration a degenerate spacetime metric would result.) In the limit, the observers measure the spacetime to have the plane-wave structure.
\end{quote}

This limiting procedure is known as the \textit{Penrose limit}. We apply it to both local and nonlocal solutions of electromagnetic and linearized gravitational theories, in spacetimes of four or more dimensions.

We consider two frames: the rest frame $\bar{S}$, in which the matter source is stationary, and the frame $S$, moving with constant velocity $\beta$ along the $\xi$-direction. We introduce coordinates adapted to this setup: $\xi$ runs along the direction of motion, and $\mathbf{x}_{\perp}$ denotes the two-dimensional transverse spatial coordinates. The coordinates in the two frames are
\begin{align}
X^{\mu}=(t,\xi, x_{\perp}^i), \quad \bar{X}^{\mu}=(\bar{t},\bar{\xi}, x_{\perp}^i)\, ,
\end{align}
where $i=1,2$. The transverse coordinates $x_\perp^i$ remain unchanged under a boost in the $\xi$-direction. The Minkowski metric takes the same form in both frames:
\begin{align}
ds_0^2 = -d\bar{t}^2 + d\bar{\xi}^2 + d\mathbf{x}_\perp^2 = -dt^2 + d\xi^2 + d\mathbf{x}_\perp^2 \, .
\end{align}
Quantities defined in the rest frame will be denoted with a bar throughout the remainder of this section. For example, the radial distance from the origin to a point $(\bar{\xi}, x_{\perp}^i)$ is $\bar{r}^2 = \bar{\xi}^2 + \mathbf{x}_\perp^2$. The coordinates $x_\perp^j$ are defined as in Section~\eqref{sect2.6}.

We now apply a boost along the $\bar{\xi}$-direction to the stationary solutions described earlier. The transformation is
\begin{align}
\label{eq:boost}
\bar{t} = \gamma(t - \beta \xi) \, , \quad
\bar{\xi} = \gamma(\xi - \beta t) \, ,
\end{align}
where $\gamma = 1/\sqrt{1 - \beta^2}$. For fixed $\xi$, the relation $\bar{\xi} = -\gamma \beta t + \text{const}$ shows that frame $S$ moves to the left (negative $\bar{\xi}$ direction) relative to $\bar{S}$, or equivalently, the pencil appears to move with positive velocity in $S$.

We introduce null coordinates in frame $S$:
\begin{align}
u = \frac{t - \xi}{\sqrt{2}} \, , \quad v = \frac{t + \xi}{\sqrt{2}} \, .
\end{align}
The boost \eqref{eq:boost} becomes
\begin{align}
\label{tx}
\bar{t} &= \frac{\gamma}{\sqrt{2}}[(1+\beta)u + (1-\beta)v] \, , \\
\bar{\xi} &= \frac{\gamma}{\sqrt{2}}[-(1+\beta)u + (1-\beta)v] \, .
\end{align}
In the ultrarelativistic limit $\beta \to 1$, these reduce to
\begin{align}
\bar{t} \to \sqrt{2}\gamma u \, , \quad \bar{\xi} \to -\sqrt{2}\gamma u \, .
\end{align}
This implies that a pencil at rest in $\bar{S}$ and occupying the region $\bar{\xi} \in [0, \bar{L}]$ is located in the boosted frame $S$ within the strip $u \in [-L/\sqrt{2}, 0]$, where $L = \bar{L}/\gamma$. See Fig.~\eqref{fig:u-strip}.

\begin{figure}[!hbt]
    \centering
    \vspace{10pt}
    \includegraphics[width=0.7\textwidth]{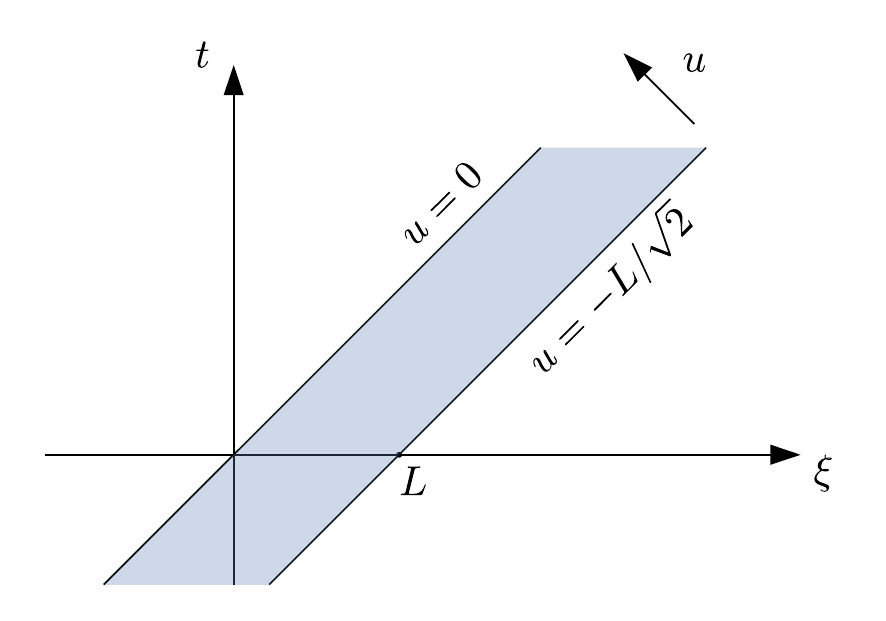}
    \caption{The pencil of length $L$ moves within the two-dimensional $(t,\xi)$-section of Minkowski space in the frame $S$.}
    \label{fig:u-strip}
\end{figure}

\subsection{Green Functions in the Penrose Limit}

As shown in previous sections, solutions for stationary sources in the rest frame $\bar{S}$ can be expressed using Green functions of the form
\begin{equation}
f(\Delta)\Delta  \mathcal{G}_d(\mathbf{x}-\mathbf{x}')=-\delta^{(d)}(\mathbf{x}-\mathbf{x}') \, ,
\end{equation}
where $f$ is the form factor of the nonlocal theory, and $d = D-1$ is the number of spatial dimensions. For the local case $f=1$, $\mathcal{G}_d = G_d$ is the standard Green function of the $d$-dimensional Laplace operator.

To analyze the Penrose limit, we rewrite the static Green function using the following representation:
\begin{align}
\label{eq:green-function-2}
\mathcal{G}_d(r) &= \frac{1}{2\pi}\int_{-\infty}^\infty \frac{d\eta}{f(-\eta \ell^2)\eta} \int_{-\infty}^\infty d\tau \, K_d(r|\tau) \, e^{i\eta \tau} \, ,
\end{align}
where
\begin{equation} 
K_d(r|\tau) = \frac{1}{(4\pi i \tau)^{\tfrac{d}{2}}} e^{i \tfrac{r^2}{4\tau}} \, ,
\end{equation}
is the $d$-dimensional heat kernel in imaginary time $\tau = -it$. It satisfies:
\begin{align}
\Delta K_d(r|\tau) &= -i\partial_\tau K_d(r|\tau) \, , \\
\lim\limits_{\tau\rightarrow 0} K_d(r|\tau) &= \delta^{(d)}(\mathbf{r}) \, .
\end{align}
This representation is particularly useful in the Penrose limit because $\bar{r}$ appears only in the exponential as $\exp[i\bar{r}^2/(4\tau)]$. Under the boost, the dominant contribution comes from the term $(\bar{\xi} - \bar{\xi}')^2$, which transforms as
\begin{equation}
\exp\left[i \gamma^2 \frac{(u - u')^2}{2 \tau} \right] \, .
\end{equation}
Taking the Penrose limit involves the identity (see also \cite{Shankar:1994})
\begin{align}
\delta(u) = \lim_{\epsilon \to 0} \frac{1}{\sqrt{2\pi i \epsilon}} e^{i \tfrac{u^2}{2\epsilon}} \, .
\end{align}
Setting $\epsilon = \tau/\gamma^2$ and applying this limit to \eqref{eq:green-function-2}, we find:
\begin{align}\label{UG}
\lim_{\gamma \to \infty} \gamma \mathcal{G}_d(\bar{r}) = \frac{1}{\sqrt{2}} \mathcal{G}_{d-1}(r_\perp) \delta(u - u') \, ,
\end{align}
where $r_\perp^2 = \delta_{ij} x^i_\perp x^j_\perp$.

Thus, in the Penrose limit, the Green function factorizes into a delta function in $u$ and a Green function in a space of one fewer spatial dimension. Importantly, this structure is universal: it holds in any dimension and for any form factor $f$.

\section{Electromagnetic Field of Ultrarelativistic Charged and Magnetized Objects}

The transformation of Green functions under the Penrose limit \eqref{UG} is the key tool for studying the fields of ultrarelativistic sources in both electromagnetic and gravitational theories. Nevertheless, the application differs slightly between the two due to the spin of the fields. The electromagnetic field has spin one and is described by a vector potential $\mathbf{A}$, while the gravitational field has spin two and is described by a rank-two tensor perturbation of the metric. Consequently, the transformations of charge and magnetic moment under boosts differ from those of energy and angular momentum in gravitational settings.

\subsection{Electromagnetic field in the Penrose limit}

We begin by considering the electromagnetic field produced by ultrarelativistic sources. For simplicity, we focus on charged and magnetized pencils whose charge and magnetic moment densities are $\delta$-localized in the transverse directions, while their profiles along the pre-boosted $\bar{\xi}$-direction are arbitrary functions of $\bar{\xi}$. Let $\bar{\lambda}(\bar{\xi})$ and $\bar{\mu}(\bar{\xi})$ denote the charge and magnetic moment line densities, respectively. More general configurations with extended transverse structure can be obtained via the superposition of these basic solutions.

Using the results derived earlier, the vector potential $\bar{A}_\mu$ for a static pencil-like distribution of charge and magnetic moment is given by
\begin{align}
\label{eq:a:pre-boost-pencil}
\bar{A}_{\bar{t}} &= \int_{-\infty}^\infty d\bar{\xi}' \, \bar{\lambda}(\bar{\xi}') \, \mathcal{G}_3(\bar{r}) \, , \\
\bar{A}_{\varphi} &= -2\pi \int_{-\infty}^\infty d\bar{\xi}' \, \mathcal{G}_{5}(\bar{r})  \bar{\mu}(\bar{\xi}') \rho^2 \, , \\
\bar{r}^2 &= (\bar{\xi}' - \bar{\xi})^2 + \rho^2  \, .
\end{align}

To study the ultrarelativistic limit, we boost this solution via the Lorentz transformation \eqref{eq:boost} and then take the limit $\gamma \to \infty$. In order to obtain finite, nontrivial expressions in this limit, we fix the total charge $q = \bar{q}$ and scale the magnetic moment as $m = \gamma \bar{m}$. Accordingly, we define the rescaled densities:
\begin{align}
\lambda(u) &= \lim_{\gamma \to \infty} \sqrt{2} \gamma \, \bar{\lambda}(-\sqrt{2} \gamma u) \, , \\
\mu(u) &= \lim_{\gamma \to \infty} \sqrt{2} \, \bar{\mu}(-\sqrt{2} \gamma u) \, .
\end{align}

Applying the transformation law \eqref{UG} for Green functions in the Penrose limit, we find that the ultrarelativistic pencil of charge and magnetic moment has the following potential:
\begin{align}
\label{eq:ultrarelativistic-pencil}
A_\mu dX^\mu = \lambda(u) \, \mathcal{G}_{2}^N(r_\perp) \, du 
- \pi \, \mathcal{G}_{4}^N(r_\perp)  \mu(u) \rho^2 \, d\varphi \, .
\end{align}
We can write this expression with explicit use of the Green functions, for example for $N=1$ where they take the form
\begin{align}
A_\mu dX^\mu = -  \frac{\mathrm{Ein}(\rho^2/4\ell^2)}{4\pi} \,  \lambda(u)du 
-  \frac{1 - e^{-\rho^2/(4\ell^2)}}{4\pi\rho^2}  \mu(u) \rho^2 \, d\varphi \, .
\end{align}
Where $\text{Ein}(x)$ is the complementary exponential integral defined via:
\begin{align}
\text{Ein}(x) &= \int_0^x \frac{1 - e^{-z}}{z} \, dz = E_1(x) + \ln x + \gamma \, , \\
E_1(x) &= e^{-x} \int_0^\infty \frac{e^{-z}}{z+x} \, dz = -\text{Ei}(-x) \, ,
\end{align}
and $\gamma \approx 0.577$ is the Euler--Mascheroni constant \cite{NIST2010}. The background metric in $(u,v)$ coordinates takes the form:
\begin{align}
\label{uv-metric}
ds^2 = -2 \, du \, dv +  d\rho^2 + \rho^2 d\varphi^2 \, .
\end{align}

Remarkably, the potential~\eqref{eq:ultrarelativistic-pencil} remains regular as $r_\perp \to 0$, in sharp contrast to the standard local Maxwell theory, where the field typically diverges at the source location.

\subsection{Properties of the solutions}

Let us now examine some of the key features of the solutions obtained in nonlocal Maxwell theory. The potential~\eqref{eq:ultrarelativistic-pencil} can be rewritten in the concise form:
\begin{align}
\label{KA}
\mathbf{A} =  \lambda(u) \, h_0(\rho) \, \boldsymbol{\zeta}_0 + \mu(u) \, h_1(\rho) \, \boldsymbol{\zeta}_1 \, ,
\end{align}
where $h_0$ and $h_1$ are some functions of $\rho$. Here, $\boldsymbol{\zeta}_{0,1}$ are Killing vectors defined as
\begin{align}
\boldsymbol{\zeta}_0 = \partial_v \, , \quad \boldsymbol{\zeta}_1 = \partial_{\varphi} \, .
\end{align}
It is straightforward to verify that
\begin{align}
\mathcal{L}_{\boldsymbol{\zeta}_i} \mathbf{A} = 0 \, ,
\end{align}
where $\mathcal{L}_{\boldsymbol{\zeta}}$ denotes the Lie derivative along $\boldsymbol{\zeta}$. These relations confirm that the ultrarelativistic solutions preserve the expected symmetries: invariance under translations in $v$ and rotations in each $\varphi$-direction.

Another important observation is that, in the absence of magnetic moment (i.e., when $\mu = 0$), the electromagnetic field is null:
\begin{align}
F_{\mu\alpha} F^\alpha{}_\nu &= S \, u_{,\mu} u_{,\nu} \, , \quad
F^2 = \frac{1}{2} F_{\mu\nu} F^{\mu\nu} = 0 \, .
\end{align}
\textit{(Note: For a static $q$-pencil of fixed length $\bar{L}$, the invariant $F^2$ is non-zero. However, in the Penrose limit, $\bar{L} \to \gamma \bar{L}$, causing $F^2$ to vanish as $\gamma \to \infty$.)}

In general, magnetic fields destroy this null structure. However, in four-dimensional spacetime, standard Maxwell theory exhibits a special case where the field remains null. To illustrate this, we can use equation \eqref{KA}, direct computation yields:
\begin{align}
F^2 = B^2 \left( \rho \, \frac{dC}{d\rho} + 2C \right)^2 \, .
\end{align}
Thus, the field is null ($F^2 = 0$) if and only if $C(\rho) = C_0 / \rho^2$, which corresponds precisely to the local Maxwell field of a charged and magnetized pencil in four dimensions. In higher dimensions, this condition no longer holds.

Importantly, in nonlocal electrodynamics, $F^2 \neq 0$ even in four-dimensional spacetime when magnetic moments are present. Hence, nonlocality modifies the null structure of the electromagnetic field, even in situations where it would otherwise be preserved in local theory.

\subsection{Boosted pencil-like sources}

The setup parallels that of Chapter~\eqref{Ch2}, with the only difference being that $\mathbf{x}_{\perp}$ now refers to the $d-1$ transverse spatial coordinates. The coordinates in both frames remain unchanged:
\begin{align}
X^{\mu} = (t, \xi, x_{\perp}^i), \quad \bar{X}^{\mu} = (\bar{t}, \bar{\xi}, x_{\perp}^i) \, ,
\end{align}
where $i = 1, \dots, d-1$. The Minkowski metric retains the same form in both frames.

As seen at the beginning of this section, the vector potential $\bar{A}_\mu$ for a static pencil-like distribution is
\begin{align}
\bar{A}_{\bar{t}} &= \int_{-\infty}^\infty d\bar{\xi}' \, \bar{\lambda}(\bar{\xi}') \, \mathcal{G}_d(\bar{r}) \, , \\
\bar{A}_{a} &= -2\pi \int_{-\infty}^\infty d\bar{\xi}' \, \mathcal{G}_{d+2}(\bar{r}) \sum_{a=1}^n \bar{\mu}_a(\bar{\xi}') \rho_a^2 \, , \\
\bar{r}^2 &= (\bar{\xi}' - \bar{\xi})^2 + \mathbf{x}_\perp^2 \, , \quad
\mathbf{x}_\perp^2 = \sum_{a=1}^n \rho_a^2 + \epsilon z^2 \, .
\end{align}

To obtain the ultrarelativistic limit, we define the rescaled densities:
\begin{align}
\lambda(u) &= \lim_{\gamma \to \infty} \sqrt{2} \gamma \, \bar{\lambda}(-\sqrt{2} \gamma u) \, , \\
\mu_a(u) &= \lim_{\gamma \to \infty} \sqrt{2} \, \bar{\mu}_a(-\sqrt{2} \gamma u) \, .
\end{align}

Using the transformation law~\eqref{UG} for the Green functions in the Penrose limit, we find the ultrarelativistic potential:
\begin{align}
\label{appeq:ultrarelativistic-pencil}
A_\mu dX^\mu = \lambda(u) \, \mathcal{G}_{d-1}^N(r_\perp) \, du 
- \pi \, \mathcal{G}_{d+1}^N(r_\perp) \sum_{a=1}^n \mu_a(u) \rho_a^2 \, d\varphi_a \, .
\end{align}

The background metric in $(u,v)$ coordinates is
\begin{align}
ds^2 = -2 \, du \, dv + \sum_{a=1}^n (d\rho_a^2 + \rho_a^2 d\varphi_a^2) + \epsilon dz^2 \, .
\end{align}
As in the $D=4$ case discussed earlier in the thesis, the potential~\eqref{appeq:ultrarelativistic-pencil} remains regular in the limit $r_\perp \to 0$.

\subsection{Properties of the solutions}

The potential~\eqref{appeq:ultrarelativistic-pencil} can be rewritten to illustrate that one of the key features remains unchanged in higher dimensions. Namely,
\begin{align}
\mathbf{A} = \sum_{a=0}^n \lambda_a(u) \, a_a(r_\perp) \, \boldsymbol{\zeta}_a \, ,
\end{align}
where $\lambda_0(u) = \lambda(u)$ and $\lambda_{a \geq 1}(u) = \mu_a(u)$. Now, $\boldsymbol{\zeta}_a$ are Killing vectors defined as
\begin{align}
\boldsymbol{\zeta}_0 = \partial_v \, , \quad \boldsymbol{\zeta}_a = \partial_{\varphi_a} \, .
\end{align}
It is straightforward to verify that
\begin{align}
\mathcal{L}_{\boldsymbol{\zeta}_a} \mathbf{A} = 0 \, ,
\end{align}
where $\mathcal{L}_{\boldsymbol{\zeta}}$ denotes the Lie derivative along $\boldsymbol{\zeta}$. Thus, invariance under translations in $v$ and rotations in each $\varphi_a$-direction remains conserved as well.

\section{Pencil-like gravitational sources in four spacetime diemensions}

As in earlier sections, we now consider an extended object with negligible transverse size but finite extent in one spatial direction. We assume it is massive and spinning about its axis. We study its gravitational field in the rest frame $\bar{S}$, where the time and longitudinal coordinates are denoted by $\bar{t}$ and $\bar{\xi}$, respectively. The flat background metric in these coordinates reads
\begin{equation}
ds^2 = -d\bar{t}^2 + d\bar{\xi}^2 + d\mathbf{x}_\perp^2 \, .
\end{equation}

To model the stress-energy tensor \eqref{TTT} for such a pencil-like configuration, we assume both the mass density $\rho$ and angular momentum density $j_{ij}$ are localized along the line defined by the pencil. We define the line densities of mass and angular momentum by $\bar{\lambda}(\bar{\xi})$ and $\bar{j}_{ij}(\bar{\xi})$, respectively. These quantities describe how mass and angular momentum are distributed along the pencil’s length. Imposing that the angular momentum is transverse to the $\bar{\xi}$-direction, so that $\bar{j}_{i\bar{\xi}}(\bar{\xi}) = 0$, the stress-energy tensor for the spinning pencil becomes
\begin{align}
\label{eq:tmunu-pencil}
T_{\mu\nu} = \left[ \delta^{\bar{t}}_\mu \delta^{\bar{t}}_\nu \, \bar{\lambda}(\bar{\xi}) +  \bar{j}(\bar{\xi}) \delta^{\bar{t}}_{(\mu} \delta^i_{\nu)} \, \epsilon^{j}_i \, \partial_j \right] \delta^{(2)}(\mathbf{x}_\perp) \, .
\end{align}

We assume that the pencil has finite length in the $\bar{\xi}$-direction, with both $\bar{\lambda}(\bar{\xi})$ and $\bar{j}_a(\bar{\xi})$ vanishing outside the interval $(0, \bar{L})$. We refer to $\bar{L}$ as the length of the pencil. The total mass and angular momentum are given by
\begin{align}
\label{eq:m-def}
\bar{m} &= \int d\bar{\xi} \, \bar{\lambda}(\bar{\xi}) \, , \\
\label{eq:j-def-1}
\bar{J}_{ij} &= \int d\bar{\xi} \, \bar{j}_{ij}(\bar{\xi}) \, , \\
\label{eq:j-def-2}
\bar{j}_{ij}(\bar{\xi}) &=  \epsilon^{}_{ij} \, \bar{j}(\bar{\xi}) \, .
\end{align}

The resulting gravitational field $h_{\mu\nu}$ generated by this source is
\begin{align}
\mathbf{h} = \bar{\phi} \left[ dt^2 +(d\bar{\xi}^2 + d\mathbf{x}_\perp^2) \right] + 2\bar{A}_i \, dx_\perp^i \, dt \, ,
\end{align}
With the potentials given by
\begin{align}
\label{SolGyr:StatGrav}
\begin{split}
\bar{\phi}(\bar{\xi}, x_\perp^i) &= \kappa  \int d\bar{\xi}' \, \bar{\lambda}(\bar{\xi}') \, \mathcal{G}_3(\bar{r}) \, , \\
\bar{A}_i(\bar{\xi}, x_\perp^i) &= -2\pi\kappa \int d\bar{\xi}' \, \bar{j}_{ij}(\bar{\xi}') \, x_\perp^j \, \mathcal{G}_{5}(\bar{r}) \, .
\end{split}
\end{align}
Here, $\bar{r}^2$ is defined in \eqref{eq:a:pre-boost}.

\section{Gravitational field of ultrarelativistic massive and spinning objects}

As previously noted, there are formal similarities between electromagnetism and linearized gravity. However, a fundamental difference arises due to the nature of their respective sources: electric charge can be positive or negative, allowing for electrically neutral but magnetized objects, whereas energy in gravity is always positive. Consequently, one cannot consider purely spin-induced gravitational fields without any accompanying energy density.

This distinction becomes relevant when modeling beams of spinning, massless particles. In such cases, the relation between energy density and spin distribution must be carefully analyzed—typically within the framework of geometric optics. However, this analysis lies beyond the scope of the present work. Instead, we concentrate on the gravitational field generated by ultrarelativistic sources in linearized gravity and its nonlocal, ghost-free generalization. Within this framework, we treat the energy and angular momentum density distributions as arbitrary.

\subsection{Scaling properties}

Let us first examine how the parameters of a spinning pencil transform under a Lorentz boost \eqref{eq:boost}. Suppose the rest-frame ($\bar{S}$) mass and angular momentum are uniformly distributed along the pencil, with linear densities $\bar{\lambda} = \bar{m}/\bar{L}$ and $\bar{j} = \bar{J}/\bar{L}$ held constant. Due to Lorentz contraction, the pencil's length in the boosted frame $S$ becomes $L = \bar{L} / \gamma$, and its energy transforms as $E = m = \gamma \bar{m}$. Thus, the energy density in the $S$ frame is $\lambda = \gamma^2 \bar{\lambda}$.

In the Penrose limit, we fix the total energy $E$, implying that $\lambda \to \infty$ as $\gamma \to \infty$. To keep the energy density finite, we rescale the rest-frame length as $\bar{L} \to \gamma \bar{L}$, so that the observed length $L$ remains constant.

\footnote{
We emphasize that this discussion does not address the physical constraints imposed on the matter generating the gravitational field. For instance, enforcing the null energy condition implies $|\bar{J}| \leq R \bar{m}$, where $R$ is the transverse size of the pencil. To maintain a fixed $|\bar{J}|$ as $\bar{m} \to 0$ without violating this condition, one must consider pencils with non-negligible transverse extension. Notably, in higher dimensions, the situation is more nuanced: Myers and Perry showed in \cite{Myers:1986un} that \textit{“for $N>5$, black holes with fixed mass may have arbitrarily large angular momentum”}, where $N$ is the number of spatial dimensions (denoted by $d$ in this work).
}

Because we hold the ratio $\bar{L}/\gamma$ constant in the Penrose limit, the energy density scales as
\begin{align}
\label{eq:pr-limit-mass}
\lambda(u) = \lim_{\gamma \to \infty} \sqrt{2} \gamma^2 \, \bar{\lambda}(-\sqrt{2} \gamma u) \, .
\end{align}
This ensures that the product $\bar{m} \gamma$ and the effective length $\bar{L}/\gamma$ remain fixed:
\begin{align}
E = \gamma \bar{m} = \gamma \int_{-\infty}^\infty d\bar{\xi} \, \bar{\lambda}(\bar{\xi}) 
= \int_{-\infty}^\infty du \, \lambda(u) = \text{const} \, .
\end{align}

The angular momentum density $\bar{j}_{ij}(\bar{\xi})$ resides in the transverse space and remains tensorially unchanged under the boost. Accordingly, the boosted angular momentum density in the $S$ frame is defined as:
\begin{align}
\label{eq:pr-limit-angular-momentum}
j_{ij}(u) &= \lim_{\gamma \to \infty} \sqrt{2} \gamma \, \bar{j}_{ij}(-\sqrt{2} \gamma u) \, , \\
j(u) &= \lim_{\gamma \to \infty} \sqrt{2} \gamma \, \bar{j}(-\sqrt{2} \gamma u) \, .
\end{align}
As a result, the total angular momentum $J$ of the pencil remains finite:
\begin{align}
J_{ij} = \int_{-\infty}^\infty d\bar{\xi} \, \bar{j}_{ij}(\bar{\xi}) = \int_{-\infty}^\infty du \, j_{ij}(u) \, .
\end{align}

\subsection{Metric}

After taking the Penrose limit as defined earlier, the resulting metric describing the ultrarelativistic spinning source (a gyraton) takes the form
\begin{align}
\begin{split}
\label{eq:gyraton-1}
\mathbf{g} &= \left(\eta_{\mu\nu} + h_{\mu\nu}\right) dX^\mu dX^\nu \\
&= -2 \, du \, dv + \phi \, du^2 + 2 A_i \, dx_\perp^i \, du + d\mathbf{x}_\perp^2 \, ,
\end{split}
\end{align}
where the potentials $\phi$ and $A_i$ are defined as the following boosted limits:
\begin{align}
\label{ffAA}
\phi = \lim_{\gamma \rightarrow \infty}  4 \gamma^2  \, \bar{\phi} \, , \quad
A_i = \lim_{\gamma \rightarrow \infty} \sqrt{2} \gamma \, \bar{A}_i \, .
\end{align}
Here, $\bar{\phi}$ and $\bar{A}_i$ are the static gravitational potentials defined in equation~\eqref{SolGyr:StatGrav}, and the integrands in their expressions involve the Green function $\mathcal{G}_d(\bar{r})$. Applying the Penrose limit to \eqref{ffAA}, and using the factorization property of the Green functions, one finds the limiting expressions:
\begin{align}
\label{eq:phi-final}
\phi(u, \mathbf{x}_\perp) &= 2\sqrt{2} \kappa \lambda(u) \, \mathcal{G}_{2}(r_\perp) \, , \\
A_i(u, \mathbf{x}_\perp) &= -2\pi \kappa \, j_{ij}(u) \, x_\perp^j \, \mathcal{G}_{4}(r_\perp) \, .
\end{align}

We can introduce the polar coordinates $\{\rho, \varphi\}$ as in Chapter \eqref{Ch2} and rewrite the combination $j_{ij} \, x_\perp^i dx_\perp^j$ using the relation
\begin{align}
\label{eq:j_ij_simplified}
j_{ij} \, x_\perp^i dx_\perp^j =  j(u) \, \rho^2 \, d\varphi_a \, .
\end{align}
This yields a compact expression for the gravitomagnetic potential one-form:
\begin{align}
\label{eq:a-final}
A_i(\mathbf{x}_\perp) dx^i_\perp = 2\pi \kappa \, \mathcal{G}_{4}(r_\perp) j(u) \rho^2 \, d\varphi \, ,
\end{align}
which makes the rotational symmetry manifest.

\section{Gravitational field of ghost-free gyratons}

Ultrarelativistic spinning sources producing the gravitational field described above are known as \textit{gyratons} (see e.g.~\cite{BHFrolZel}). In this section, we explore gyraton-like solutions both in General Relativity and in ghost-free (nonlocal) gravity.

In General Relativity, the form factor is trivial:
\begin{align}
f(\Box) = 1 \, ,
\end{align}
whereas in ghost-free gravity theories denoted $\mathrm{GF}_N$, the form factor takes the nonlocal exponential form
\begin{align}
\label{eq:form-factor-gfn}
f(\Box) = \exp\left[(-\Box \ell^2)^N\right] \, .
\end{align}
The static Green function \eqref{NLGreen} can be computed for a wide class of such theories. In this thesis, we focus on General Relativity as well as on two infinite-derivative models with $N = 1$ and $N = 2$, denoted respectively by $\mathrm{GF}_1$ and $\mathrm{GF}_2$. These results are readily generalizable to any number of spatial dimensions $d$.

\subsection{Gyratons in d = 3}

\subsubsection{Gyraton metrics in General Relativity}

As a preliminary example, consider the well-known $(3+1)$-dimensional gyraton solutions of General Relativity \cite{Bonnor1969,Bonnor:1969rb,Frolov:2005in,Frolov:2005zq}. The relevant static Green functions are:
\begin{align}
G_2(r) = -\frac{1}{2\pi} \log(r) \, , \quad
G_4(r) = \frac{1}{4\pi^2 r^2} \, .
\end{align}
In $d=3$, the transverse space is two-dimensional, so we set $n=1$ and $\epsilon=0$. Denoting the radial coordinate as $\rho = |\mathbf{x}_\perp|$, the polar angle as $\varphi$, and the angular momentum density in the $S$ frame as $j(u)$, the gravitational potentials become:
\begin{align}
\phi(u,\rho) &= -\frac{\sqrt{2} \kappa \lambda(u)}{2\pi} \log(\rho) \, , \\
\mathbf{A}(u) &= \frac{\kappa j(u)}{2\pi} \, d\varphi \, .
\end{align}
The corresponding gravitomagnetic field is locally exact:
\begin{align}
\mathbf{F} = d\mathbf{A} = 0 \, .
\end{align}
Nevertheless, the total gravitomagnetic charge is nonzero:
\begin{align}
Q_0 = \int_{\mathcal{A}} \mathbf{F} = \oint_{\partial \mathcal{A}} \mathbf{A} = \kappa j(u) \, ,
\end{align}
where $\mathcal{A}$ is any surface in the transverse plane (e.g., a circle of radius $\rho$). In linearized General Relativity, this charge is conserved across all contours in a given null plane $u = \text{const}$. As we will show, this property breaks down in nonlocal gravity, where the gravitomagnetic current becomes spatially smeared in the transverse direction.

\subsubsection{Gyraton metrics in ghost-free gravity}

We now consider analogous solutions in ghost-free gravity. For the $\mathrm{GF}_1$ model, the two-dimensional Green function reads:
\begin{align}
\mathcal{G}_2(r) = -\frac{1}{4\pi} \, \text{Ein}\left(\frac{r^2}{4\ell^2}\right) \, .
\end{align}

The gravitational potentials then take the form:
\begin{align}
\phi(u,\rho) &= -\frac{\sqrt{2} \kappa \lambda(u)}{2\pi} \, \text{Ein}\left(\frac{\rho^2}{4\ell^2}\right) \, , \\
\mathbf{A}(u,\rho) &= \frac{\kappa j(u)}{2\pi} \left[1 - \exp\left(-\frac{\rho^2}{4\ell^2}\right)\right] d\varphi \, .
\end{align}
The gravitomagnetic field is no longer exact, and the corresponding charge becomes radius-dependent:
\begin{align}
Q_1(\rho) = \kappa j(u) \left[1 - \exp\left(-\frac{\rho^2}{4\ell^2}\right)\right] \, .
\end{align}
At large distances $\rho \gg \ell$, the solution asymptotes to that of General Relativity.

In the $\mathrm{GF}_2$ model, the Green function is given by:
\begin{align}
\begin{split}
\mathcal{G}_2(r) &= \frac{y}{2\pi} \left[\sqrt{\pi} \, {}_1F_3\left(\tfrac{1}{2}; 1, \tfrac{3}{2}, \tfrac{3}{2}; y^2\right) \right. \\
&\left. \hspace{30pt} - y \, {}_2F_4\left(1,1; \tfrac{3}{2}, \tfrac{3}{2}, 2, 2; y^2\right) \right] \, ,
\end{split}
\end{align}
with $y = \rho^2 / (16\ell^2)$. The corresponding gravitomagnetic charge is:
\begin{align}
\begin{split}
Q_2(\rho) &= -\kappa j(u) \left[1 - {}_0F_2\left(\tfrac{1}{2}, \tfrac{1}{2}; y^2\right) \right. \\
&\left. \hspace{40pt} - 2\sqrt{\pi} y \, {}_0F_2\left(1, \tfrac{3}{2}; y^2\right) \right] \, .
\end{split}
\end{align}

\subsubsection{Curvature invariants}

It is instructive to examine the geometric properties of the four-dimensional gyraton spacetime,
\begin{align}
\begin{split}
\mathbf{g} &= -2 \, d u \, d v + \phi(u,x,y) \, d u^2 + d x^2 + d y^2 \\
&\hspace{12pt} + 2 \left[ A_x(u,x,y) \, d x + A_y(u,x,y) \, d y \right] d u \, .
\end{split}
\end{align}
This spacetime belongs to the class of pp-wave geometries, characterized by the existence of a covariantly constant null Killing vector $\mathbf{k} = \partial_v$ \cite{Stephani:2003tm},
\begin{align}
\nabla_\nu k^\mu = 0 \, .
\end{align}
This property holds regardless of the specific form of the functions $\phi$, $A_x$, and $A_y$, provided their dependence on coordinates follows the same structure. 

A notable feature of pp-wave spacetimes is that all scalar polynomial curvature invariants vanish identically:
\begin{align}
R = R_{\mu\nu} R^{\mu\nu} = R_{\mu\nu\rho\sigma} R^{\mu\nu\rho\sigma} = 0 \, .
\end{align}
Consequently, such curvature invariants are unaffected by the transition from linearized General Relativity to its nonlocal, infinite-derivative extensions.

Now, in this section, we turn to Chapter~\eqref{Ch3} and recast the construction of the solutions for gravitational gyratons in an arbitrary number of dimensions.

\section{Higher dimensional gravitational point-like and pencil-like sources}

\subsection{Higher-dimensional Pencil-like Gravitational Source}

In order to define the stress-energy tensor of the source, we impose the following constraints on the structure of $\bar{j}_{ij}(\bar{\xi})$:
\begin{itemize}
    \item The angular momentum is entirely transverse to the $\bar{\xi}$-direction: $\bar{j}_{i\bar{\xi}}(\bar{\xi}) = 0$;
    \item The eigen two-planes $\Pi_a$ of $\bar{j}_{ij}(\bar{\xi})$ are parallel transported along the $\bar{\xi}$-axis.
\end{itemize}

These conditions allow $\bar{j}_{ij}(\bar{\xi})$ to be written in a block-diagonal form:
\begin{align}
\mathbf{\bar{j}} \hat{=} \begin{pmatrix}
0 & \bar{j}_1 & & & \dots & & & 0 \\
-\bar{j}_1 & 0 & & & & & & \\
& & 0 & \bar{j}_2 & & & & \\
& & -\bar{j}_2 & 0 & & & & \\
\vdots & & & & \ddots & & & \\
& & & & & 0 & \bar{j}_n & \\
& & & & & -\bar{j}_n & 0 & \\
0 & & & & & & & 0
\end{pmatrix} ,
\end{align}
where each $\bar{j}_a$ is a function of $\bar{\xi}$ alone.

We further decompose the $(d-1)$ transverse coordinates $x_\perp^j$ as
\begin{align}
\begin{split}\label{eq:d-epsilion}
x_\perp^j &= (y^a, \hat{y}^a, \epsilon z) \, , \quad a = 1,\dots,n \, , \\
n &= \left\lfloor \frac{d-1}{2} \right\rfloor \, , \quad d = 2n + 1 + \epsilon \, ,
\end{split}
\end{align}
where the transverse space is formed by $n$ mutually orthogonal two-planes $\Pi_a$ with right-handed coordinates $(y^a, \hat{y}^a)$, called \emph{Darboux planes}. If the spacetime dimension $d+1$ is odd, then $\epsilon = 1$ and the $z$-direction provides an additional axis orthogonal to all $\Pi_a$ and to $\bar{\xi}$. In even dimensions, this extra direction is absent.

We define the basis vectors $\mathbf{e}^{(a)} = \partial_{y^a}$ and $\hat{\mathbf{e}}^{(a)} = \partial_{\hat{y}^a}$, and their dual 1-forms $\omega^{(a)} = dy^a$, $\hat{\omega}^{(a)} = d\hat{y}^a$. The area 2-form on each Darboux plane is then
\begin{align}
\epsilon^{(a)} = \omega^{(a)} \wedge \hat{\omega}^{(a)} \, .
\end{align}

In these coordinates, the stress-energy tensor for the spinning pencil becomes
\begin{align}\label{appeq:tmunu-pencil}
T_{\mu\nu} = \left[ \delta^{\bar{t}}_\mu \delta^{\bar{t}}_\nu \, \bar{\lambda}(\bar{\xi}) + \sum_{a=1}^{n} \bar{j}_a(\bar{\xi}) \delta^{\bar{t}}_{(\mu} \delta^i_{\nu)} \, \epsilon^{(a)j}_i \, \partial_j \right] \delta^{(d-1)}(\mathbf{x}_\perp) \, .
\end{align}

We make the same assumptions as in Chapter~\eqref{Ch3}, but now define
\begin{align}
\bar{j}_{ij}(\bar{\xi}) &= \sum_{a=1}^n \epsilon^{(a)}_{ij} \, \bar{j}_a(\bar{\xi}) \, .
\end{align}

The resulting gravitational field $h_{\mu\nu}$ generated by this source is
\begin{align}
\mathbf{h} = \bar{\phi} \left[ dt^2 + \frac{1}{d-2} (d\bar{\xi}^2 + d\mathbf{x}_\perp^2) \right] + 2\bar{A}_i \, dx_\perp^i \, dt \, ,
\end{align}
with the potentials given by
\begin{align}
\begin{split}
\bar{\phi}(\bar{\xi}, x_\perp^i) &= 2\kappa \frac{d-2}{d-1} \int d\bar{\xi}' \, \bar{\lambda}(\bar{\xi}') \, \mathcal{G}_d(\bar{r}) \, , \\
\bar{A}_i(\bar{\xi}, x_\perp^i) &= -2\pi\kappa \int d\bar{\xi}' \, \bar{j}_{ij}(\bar{\xi}') \, x_\perp^j \, \mathcal{G}_{d+2}(\bar{r}) \, .
\end{split}
\end{align}
Here, $\bar{r}^2$ is defined in~\eqref{app-radiusdef}.

\subsection{Metric and Scaling Properties}

The properties of the angular momentum density $\bar{j}_{ij}(\bar{\xi})$ remain unchanged. To proceed, we define the boosted angular momentum profile via
\begin{align}
j_a(u) = \lim_{\gamma \to \infty} \sqrt{2} \gamma \, \bar{j}_a(-\sqrt{2} \gamma u) \, .
\end{align}

After performing the Penrose limit, the resulting metric retains its pp-wave structure:
\begin{align}
\begin{split}
\mathbf{g} &= \left(\eta_{\mu\nu} + h_{\mu\nu}\right) dX^\mu dX^\nu \\
&= -2 \, du \, dv + \phi \, du^2 + 2 A_i \, dx_\perp^i \, du + d\mathbf{x}_\perp^2 \, ,
\end{split}
\end{align}
but the gravitational potentials $\phi$ and $A_i$ now scale as
\begin{align}\label{appffAA}
\phi = \lim_{\gamma \rightarrow \infty} 2 \gamma^2 \frac{d-1}{d-2} \, \bar{\phi} \, , \quad
A_i = \lim_{\gamma \rightarrow \infty} \sqrt{2} \gamma \, \bar{A}_i \, .
\end{align}

Applying the Penrose limit to Eq.~\eqref{appffAA} and using the factorization properties of the Green functions yields
\begin{align}
\label{appeq:phi-final}
\phi(u, \mathbf{x}_\perp) &= 2\sqrt{2} \kappa \lambda(u) \, \mathcal{G}_{d-1}(r_\perp) \, , \\
A_i(u, \mathbf{x}_\perp) &= -2\pi \kappa \, j_{ij}(u) \, x_\perp^j \, \mathcal{G}_{d+1}(r_\perp) \, .
\end{align}

Introducing polar coordinates $\{\rho_a, \varphi_a\}$ in each Darboux plane $\Pi_a$ via
\begin{align}
y^a = \rho_a \cos\varphi_a \, , \quad \hat{y}^a = \rho_a \sin\varphi_a \, ,
\end{align}
the combination $j_{ij} \, x_\perp^i dx_\perp^j$ can be rewritten as
\begin{align}
j_{ij} \, x_\perp^i dx_\perp^j = \sum_{a=1}^n j_a(u) \, \rho_a^2 \, d\varphi_a \, ,
\end{align}
so that the gravitomagnetic one-form becomes
\begin{align}
A_i(\mathbf{x}_\perp) dx^i_\perp = 2\pi \kappa \, \mathcal{G}_{d+1}(r_\perp) \sum_{a=1}^n j_a(u) \rho_a^2 \, d\varphi_a \, ,
\end{align}
making the rotational symmetry in each Darboux plane manifest.

\subsection{Gyratons in Four and Higher Spatial Dimensions}

\subsubsection*{The Case $d = 4$}

In five spacetime dimensions, corresponding to $d=4$, we have $n=1$ and $\epsilon=1$, implying the presence of a single Darboux plane orthogonal to the boost direction $\xi$, along with an additional $z$-axis. Introducing the transverse radius $r_\perp$ via
\begin{align}
r_\perp^2 = \rho^2 + z^2 \, ,
\end{align}
where $\rho$ is the radial coordinate in the Darboux plane, the gravitational potentials follow from Eqs.~\eqref{appeq:phi-final} and \eqref{eq:a-final}:
\begin{align}
\phi &= 2\sqrt{2}\kappa\lambda(u)\mathcal{G}_3(r_\perp) \, , \\
A_i dx_\perp^i &= -\frac{\kappa}{r_\perp} \frac{d}{dr_\perp} \mathcal{G}_3(r_\perp) j(u) \rho^2 d\varphi \, ,
\end{align}
where $\varphi$ denotes the polar angle in the Darboux plane, $j(u)$ encodes the angular momentum profile, and $\lambda(u)$ the energy density along the null direction. Explicit expressions for the Green function $\mathcal{G}_3$ in General Relativity and ghost-free theories $\mathrm{GF}_1$ and $\mathrm{GF}_2$ can be found in~\cite{pinedo2022gravitational}.

\subsubsection*{Higher-Dimensional Cases}

In higher dimensions, gyraton solutions can be constructed analogously. Rather than repeating the full derivation, we outline a general procedure applicable to arbitrary spatial dimension $d$:

\begin{enumerate}
    \item Determine the number of Darboux planes $n$ from $d$ using Eq.~\eqref{eq:d-epsilion}. If $d$ is even, then $\epsilon = 1$ and there exists an extra $z$-axis; if $d$ is odd, then $\epsilon = 0$.

    \item Introduce polar coordinates $\{\rho_a, \varphi_a\}$ in each Darboux plane $\Pi_a$, where $a = 1, \dots, n$. These angles are chosen to be right-handed with respect to the direction of motion.

    \item Define the squared transverse distance as
    \begin{align}
    r_\perp^2 = \sum_{a=1}^n \rho_a^2 + \epsilon z^2 \, .
    \end{align}
    This quantity serves as the argument of the Green functions in Eqs.~\eqref{appeq:phi-final} and \eqref{eq:a-final}. The Green functions $\mathcal{G}_d(r_\perp)$ in higher dimensions may be obtained via the recursion relation~\eqref{eq:ch2:recursion}.

    \item Given initial profiles $\bar{\lambda}(\bar{\xi})$ and $\bar{j}_a(\bar{\xi})$ in the rest frame, compute the corresponding null-time profiles $\lambda(u)$ and $j_a(u)$ using Eqs.~\eqref{eq:pr-limit-mass} and \eqref{eq:pr-limit-angular-momentum}.
\end{enumerate}

In realistic scenarios, gyratons may exhibit finite transverse extent. Nevertheless, owing to the linearity of the field equations, the gravitational field of such ``thick gyratons'' can be constructed by superposing the solution for point-like sources with an appropriate transverse profile added to Eq.~\eqref{appeq:tmunu-pencil}.
